# Supplementary material for: PHEW: Constructing Sparse Networks that Learn Fast and Generalize Well without Training Data
Source: arXiv:2010.11354 source file (2021-06-23)
Supplement: Supplementary file 1 [file Structural_Analysis.tex]

\section{Structural analysis}\label{strana}

%In this section we report on a structural analysis of other pruning strategies compared to PHEW. 
%We first present results for the number of remaining units at a layer as the density increases. Second, we present the layer-wise density of sparse networks obtained through various methods.

%\subsection{Layer width analysis with varying density} 

%We showed in the main body of the paper (Section 3) that subnetworks generated  using SynFlow and SynFlow-L2 result in very narrow layers.
%Further, all the hidden layers have almost the same number of remaining units.
%The major cause behind such "narrowing" of the pruned architectures is the maximization of the number of input-output paths.
%We showed that SynFlow and SynFlow-L2 networks form the highest number of input-output paths in the previous section:
%\textit{Given a target density $\rho$, the maximum number of paths results when each hidden-layer has the same number of units, and the network is fully-connected.}

%Therefore, the largest width decrease is expected at the widest layer of the unpruned network.
%In Figure \ref{widthvsdensityfigure}, we compare the number of remaining units at the layer that contains the highest number of units in the unpruned network.
%We can observe that as the density decreases the drop in the number of remaining units for subnetworks obtained through SynFlow and SYnFLow-L2 is significantly larger than other methods. 
%Further, PHEW maintains the same number of units as the unpruned network, until the network density becomes extremely low. 

%\subsection{Per-layer density}

In Figure \ref{layerwiseratio}, we plot the per-layer density of the pruned subnetworks obtained using various methods for a specific network density.
The network density is the lowest possible such that the method of Magnitude-Pruning (that can be performed only after training) achieves within 5\% of the unpruned network’s accuracy.
The layers are numbered from $1$ to $L$, where $L$ is the total number of parametrized layers, including the output layer.

\textbf{Data-dependent methods:} We can observe in Figure \ref{layerwiseratio}, that the data-dependent methods tend to eliminate more connections in the early layers than other methods. 
The major cause behind this phenomenon is explained in \cite{wang2020picking}: early convolutional layers usually learn highly sparse features, which does not require a large number of connections. As a result, early layers end up with lower density for these methods. 

\textbf{Path-based methods:} In Figure \ref{layerwiseratio}, we can observe that the path-based methods (PHEW, SynFlow and SynFlow-L2) have different per-layer densities. 
However, these methods follow the same trend across various layers. 
An interesting observation here is that these methods follow a step-like function, where the density remains the same for all hidden layers with the same unpruned width.
Further, the widest layers of the unpruned networks have the lowest density after pruning.

In PHEW, the conserved connections are selected by random walks. In each walk the same number of connections are chosen in each layer. 
Therefore, we expect the PHEW sub-network to have the same number of active connections in each layer.
As the per layer density is inversely proportional to the layer-width and the number of connections are expected to be the same for all layers, we expect the widest layer to have the lowest density.
