# Supplementary material for: PHEW: Constructing Sparse Networks that Learn Fast and Generalize Well without Training Data
Source: arXiv:2010.11354 source file (2021-06-23)
Supplement: Supplementary file 2 [file MPKT.tex]

\subsection{Maximum path kernel trace}

We consider a single hidden-layer network, $\bm{f}:\R^D\rightarrow \R^D$, with $N$ hidden units and $D$ inputs and outputs. The incoming and outgoing weights of each hidden unit are initialized by sampling from $\mathcal{N}(0,1)$. The number of connections in the unpruned network is $M$, 
while the target number of connections in the pruned network is $m<M$. The corresponding network density is $\rho = m/M$.

Using the notation of Section~2, the path kernel trace maximization problem is to select the $m$ edges that form a set of paths $P$ such that the following function is maximum: 
\begin{equation}
    \sum_{p=1}^P \sum_{i=1}^m \left(\dfrac{\pi_{p}(\bm{\theta})}{\theta_{i}}\right)^2 p_i, \mbox{~given~} m = \rho \times M
\end{equation}

We now show that  {\em this maximization results in a fully-connected network in which only $n \leq $N of the hidden-layer units remain in the pruned network -- all other units and their connections are removed. }
This also means that {\em given a target network density, the network that maximizes the path kernel trace has the narrowest possible hidden-layer width. }

\textbf{Proof:} Let us consider a path $p$ defined by the set of edge-weights $\{\theta_p^{[1]}, \theta_p^{[2]} \}$ at the first and second hop, respectively.
We can re-write the optimization problem as,
\begin{equation}
    \max \sum_{p=1}^P \left[(\theta_p^{[1]})^2 + (\theta_p^{[2]})^2\right], \mbox{~given~} m = \rho \times M
\end{equation}

For simplicity, assume that $m$ is such that we can form a fully-connected network with $n$ hidden units.

The incoming and outgoing weights of every hidden unit are sampled from the same distribution, and so we can assume that the sum of the highest d (out of D) squared weights of a unit is approximately the same across all units — for both incoming and outgoing connections. Specifically, 
let $\{\theta^{[1]}(j,i)\}_{i=1}^d$ and $\{\theta^{[2]}(k,j)\}_{k=1}^d$ be the top-d incoming and outgoing edge-weight magnitudes for a hidden-layer unit $j$, respectively. 
The previous assumption can be stated mathematically as: $\sum_{i=1}^d (\theta^{[1]}(j,i))^2 \approx \sum_{k=1}^d (\theta^{[2]}(k,j))^2$ for all $j=1,...,N$, and $\sum_{i=1}^d (\theta^{[1]}(j,i))^2 \approx \sum_{i=1}^d (\theta^{[1]}(l,i))^2$ for all $j,l = 1,...,N$. 
%This approximation is valid due to the low variance in the sample means of top-d edge-weight squares. The sample mean of top-d edge-weight squares would have a variance inversely proportional to $d$. 
%At moderate density values, we expect the value of $d$ to be close to $D$.

% write a justification here in terms of sample distribution mean and its variance.

The trace of the path kernel increases with the number of paths, and with the squared weights of the edges participating in these paths. 
Based on the previous assumption, a subnetwork that maximizes the path kernel trace is such that only $n\leq N$ units are active and each of them has $d\leq D$ incoming and outgoing edges. 
The edges are the top-d edges in terms of their squared weights. 
The number of incoming edges is the same with the number of outgoing edges because that maximizes the number of paths through the unit (product of incoming and outgoing edges). 

The optimization problem now can be re-framed as, 
\begin{equation}
    \argmax_{n,d} \sum_{j=1}^n \left\{ \sum_{i=1}^d \sum_{k=1}^d \left[(\theta^{[1]}(j,i))^2 + (\theta^{[1]}(k,j))^2 \right] \right\}
\end{equation}
\begin{equation}
    \argmax_{n,d} \left\{n \sum_{i=1}^d \sum_{k=1}^d \left[(\theta_{(i)})^2 + (\theta_{(k)})^2\right] \right\}
\end{equation}
\begin{equation}
    \argmax_{n,d} \left\{2nd \sum_{i=1}^d  \left[\theta_{(i)}\right]^2\right\}
\end{equation}
Substituting $n=m/(2\,d)$, we can find the optimal value of $d$:
\begin{equation}
   d^* = \argmax_{d} \left\{m \sum_{i=1}^d  \left[\theta_{(i)}\right]^2\right\}, \; d\leq D
\end{equation}
As $d$ increases so does the sum $\sum_{i=1}^d  [\theta_{(i)}]^2$ because $m$ is a constant. Therefore the  objective in the previous equation is maximized when $d$ takes the largest possible value $D$. That is $d^* = D$.

 The optimal width of the hidden layer is $n^* = m/(2D)$, which is the lowest possible width, given the target number of edges $m$. Finally, $P^* = n\times D^2$ is the maximum possible number of paths, given $m$.
