# Supplementary material for: PHEW: Constructing Sparse Networks that Learn Fast and Generalize Well without Training Data
Source: arXiv:2010.11354 source file (2021-06-23)
Supplement: Supplementary file 3 [file Num_Paths.tex]

\subsection{Maximizing the Number of paths}\label{sec-numpaths}

\textit{Given a target density $\rho$, the maximum number of paths results when each hidden-layer has the same number of units, and the network is fully-connected.}

\textbf{Proof :} Let us consider a $L$ layer ReLU network, $f:\R^D\rightarrow \R^K$, with $N_l$ hidden layer neurons, where $l=1,...,L-1$ .
Let the number of connections in the unpruned network be $M$, 
and let $m$ be the number of connections to be selected according to the target network density $\rho$.

We constraint the sparse network such that all the input units must have at-least one out-going connection and all the output units must have at-least one incoming connection.
The proof is divided into two segments. First we show that for a 2-layered network given $m$, number of paths is maximized by selecting $n\leq N$ neurons such that these neurons are connected to all input and output units, that is fully-connected. 
Using the first we segment we now know that the number of paths is maximized by selecting a sub-set of neurons at each layer such that network is fully-connected. 
We then show that the number of paths is maximized by selecting layer-wise same number of neurons.

\subsubsection{2-Layer Network} 
Let the number of layer $L$ be 2 and the $N_1=N, N_2=K$. 
Let the number of incoming and out-going connections for a neuron indexed as $i$ be $\{d_i,k_i\}_{i=1}^N$. 
Then the number of paths is given by, $P = \sum_{i=1}^N d_i\times k_i$ and the optimization problem is,
\begin{equation}
    \argmax \sum_{i=1}^N d_i\times k_i, \; s.t \;\sum_{i=1}^N d_i + k_i = m
\end{equation}
Without the loss of generality we can assume that $D=K$ (Explained after the proof).

Now let us consider $n\leq N$ such that, $n$ neurons are connected to all the input units as well as output units, that is they are fully-connected with $m = n(D+K) = 2nD$ edges. Such a network would have number of paths, $P^* = n\times D\times K = n\times D^2$. 

\textbf{Proof by induction :} Let us consider now that $n+a, a=1$ neurons are active, we can see that the network would no longer be fully-connected. 
We will maximize the number of paths in such a network and show that the resulting number of paths is less than $P^*$.
It is to be noted that as $n+1$ neurons are active, all $n+1$ neurons have at-least one incoming and one outgoing connection.

Let us start with the fully-connected network with $n$ neurons and $D$ incoming and outgoing connections per neuron. 
Let us consider $s_i$ such that $s_i$ connections are shifted from neuron $i$ to the $(n+1)^{th}$ neuron. 
So the number of incoming and outgoing connection through $n$ neurons becomes $\{d_i,k_i\}_{i=1}^n$.
The number of paths through a neuron $d_i\times k_i$, would be maximized when $d_i = k_i$, so we can re-write the number of paths through a neuron as $(D-s_i/2)\times (D-s_i/2)$ and number of paths through $(n+1)^{th}$ neuron becomes $(\sum_{i=1}^n (s_i/2))\times (\sum_{i=1}^n (s_i/2))$. 
The total number of paths is,
\begin{equation}
    P = \sum_{i=1}^n \left(D-\dfrac{s_i}{2}\right)^2 + \left(\sum_{i=1}^n \dfrac{s_i}{2}\right)^2 
\end{equation}
\begin{equation}
    P = n\times D^2 + \sum_{i=1}^n \left( \left[\dfrac{s_i}{2}\right]^2 -2D\dfrac{s_i}{2} \right)  + \left(\sum_{i=1}^n \dfrac{s_i}{2}\right)^2 
\end{equation}
\begin{equation}
  = P^* + \sum_{i=1}^n \left( \left[\dfrac{s_i}{2}\right]^2 -D\dfrac{s_i}{2} \right)  + \left(\sum_{i=1}^n \dfrac{s_i}{2}\right) \left(\sum_{j=1}^n \dfrac{s_j}{2} - D\right) 
\end{equation}

We know that $\sum_{i=1}^n \dfrac{s_i}{2} \leq D$ and both the second and third term of the equation are $\leq 0$. Therefore, we can conclude that $P\leq P^*$.

\textbf{Induction hypothesis :} Not let us assume that for number of neurons $n+a-1 = N-1$ and given number of connections $m=2nD$, the number of paths is maximized by the $n$ neurons active which are fully-connected. 

Let us now consider $n+a=N$ neurons. We know that the network with $N-1$ neurons has maximum number of paths when $n$ neurons are fully-connected and the rest have no connections. We can repeat the steps above, starting with $n$ fully-connected neurons and shifting connection to the $N^{th}$ neuron and show that the resulting number of paths $P\leq P^*$. 
Therefore we conclude here that for a network with single hidden layer and a given target number of edges to be selected, the number of paths is maximized by a network with a small subset of active fully-connected neurons.

\subsubsection{Layer-wise number of active neurons} 

Using the first we segment we now know that the number of paths is maximized by selecting a sub-set of neurons at each layer such that network is fully-connected. 
We now show that the number of paths is maximized by selecting layer-wise same number of neurons $n$.

Let us assume that given the parameter constraint $m$, there exists $n$ such that, there are $n$ active neurons in each of the hidden layer which are connected to all the $n$ neurons in the next as well as previous layer. 
Hence, this defines a fully connected constant width network with $n$ as the width. In such a network, $m = n\times(D+K+(L-2)n)$ and the number of paths $P^* = D\times n^{(L-1)} \times K$.
We will prove that this is the maximum number of paths possible given the parameter constraint $m$.

\textbf{Proof by Induction :} Let us consider the network has just one hidden layer, that is $L=2$. In the previous sub-section we showed that the number of paths is maximized by selecting a sub-set of neurons such that the network is fully-connected.

\textbf{Two hidden layers :} Let us not consider the network with two hidden layers. We know that the maximum number of paths result when $n_1$ neurons are active in the first layer and $n_2$ neurons are active in the second hidden layer, such that the network is fully connected. We now show that $n_1=n_2=n$. 

The optimization problem for maximizing the number of paths $P$ can be written as,
\begin{equation}
    \argmax_{n_1,n_2} P, \; s.t \; m = D n_1 + n_1 n_2 + K n_2
\end{equation}
Without the loss of generality we can assume that $D=K$ (Explained after the proof). Therefore, $P = D^2\times n_1 \times n_2$.
\begin{equation}
    \argmax_{n_1,n_2} D^2\times n_1 \times n_2, \; s.t \; m = D( n_1 +  n_2 ) + n_1 n_2 
\end{equation}
Substituting for $n_2$ from the constraint, 
\begin{equation}
   \argmax_{n_1} D^2 \times n_1 \times \dfrac{m-Dn_1}{D+n_1}
\end{equation}
Differentiating the equation and equating it to $0$, we obtain $n_1 = -D + \sqrt{D^2+m}$. Similarly, substituting and solving for $n_2$ we obtain $n_2 = -D + \sqrt{D^2+m} = n_1$. We can see here that the number of paths is maximized by having the same number of neurons $n = n_1 = n_2$, in the hidden layers.

\textbf{L layers : } The induction hypothesis on a network with $L-1$ layer is, given the target number of connections $m$, the number of paths for a network with $L-1$ layers is maximized by considering a fully-connected network with the same number of neurons in each of the hidden layer, $n\leq N_i, i=1,...,L-2$, and $m = n(D+K+(L-1)n)$.

Now let us consider a network with $L$ layers, from the induction hypothesis we know that the number of paths till the last hidden layer is maximized when each hidden layer contains the same number of active neurons and is fully-connected. Let the number of neurons in the last hidden layer to be selected be $n_{L-1}\leq N_{L-1}$. Using the same proof as above for the last hidden layer, we can conclude that the number of neurons selected in all the hidden layers will be the same.

Therefore, given a target number of connections $m$, the number of input-output paths is maximized by a sub-network such that it has the same number of active neurons $n$ in all the hidden layers and the sub-network is fully-connected.

\textbf{Assumption :} In this proof we assumed that the number of input units $D$ and the number of output units $K$ are the same. Here we show that we can make this assumption without the loss of generality. The set of input units and output units can be divided into subsets of equal number of units, where the number of units in a set is the highest common factor. As the intersection of any two subsets is a null set, maximizing the number of paths from all such sets of input units to all sets of output units is equivalent to maximizing the total number of input-output paths.

%For example, let the index set $D$ be divided into $n$ subsets containing the same number of units $\{D_i\}_{i=1}^n$ and let the index set $K$ be divided into $m$ subsets containing the same number of units $\{K_i\}_{i=1}^m$. Such that, $|D_i|=|K_j|, \forall i = 1,...,n \; , j = 1,...,m$ and $D_i\cap D_j = \emptyset, \forall i,j = 1,...,n, i\neq j$, $K_i\cap K_j = \emptyset, \forall i,j = 1,...,m, i\neq j$.
