# Supplementary material for: PHEW: Constructing Sparse Networks that Learn Fast and Generalize Well without Training Data
Source: arXiv:2010.11354 source file (2021-06-23)
Supplement: Supplementary file 4 [file PHEW_Layer_collapse.tex]

\subsection{PHEW and Layer-Collapse}\label{phewlayercollapse}

Layer collapse is defined as the network state after pruning, such that all the connections of a specific layer are eliminated, while there exists multiple connections in other layers \cite{tanaka2020pruning}.
Layer collapse causes a break of information flow through the network making the network untrainable.
The minimum network density ($\rho$) achievable without causing layer collapse is given by $\rho_{min} = L/M$, where $L$ is the number of layers and $M$ is the number of weights in an unpruned network.

\textbf{Theorem 4 :} \textit{Given a neural network architecture and a target network density $\rho$, a method that selects and conserves input-output paths achieves minimum network density $\rho_{min} = L/M$ without causing layer collapse.}

\textbf{Proof : } We will prove this theorem by considering the lower bound of the path-conservation based algorithms. The minimum number of paths that can be selected such that the sparse network avoids layer collapse is one. The number of connections added to the network is $L$, where $L$ is the number of layers. Therefore, the network density $\rho = L/M$, which is the lowest possible network density possible while avoiding layer-collapse. We conclude that a method that selects and conserves input-output paths achieves minimum network density without causing layer collapse.
