# Supplementary material for: PHEW: Constructing Sparse Networks that Learn Fast and Generalize Well without Training Data
Source: arXiv:2010.11354 source file (2021-06-23)
Supplement: Supplementary file 5 [file PHEW_PKT.tex]

% \begin{figure*}
%\centering
%        \begin{subfigure}[b]{1\textwidth}
%             \centering
%             \includegraphics[width=\textwidth]{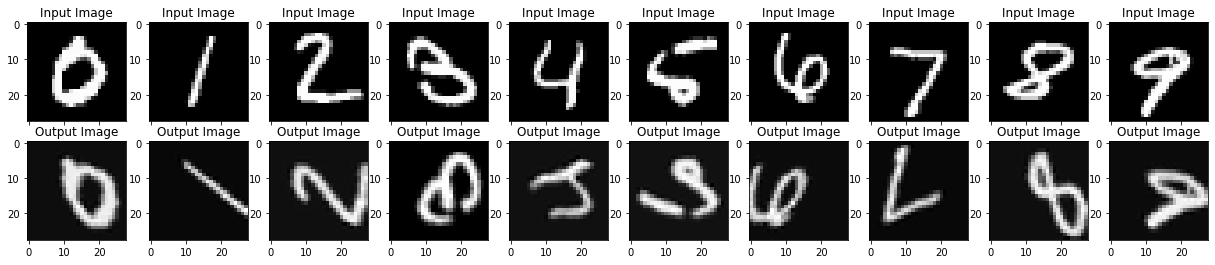}
%         \end{subfigure}
%\caption{Examples of input and output images for the transformation task}
%    \label{fig:10}
%\end{figure*}
%\begin{figure*}
%\centering
%        \centering
%         \begin{subfigure}[b]{0.245\textwidth}
%             \centering
%             \includegraphics[width=\textwidth]{Figures/Appendix/phewwidth100.png}
%         \end{subfigure}
%           \centering
%         \begin{subfigure}[b]{0.245\textwidth}
%             \centering
%             \includegraphics[width=\textwidth]{Figures/Appendix/phewwidth200.png}
%         \end{subfigure}
%         \centering
%         \begin{subfigure}[b]{0.245\textwidth}
%             \centering
%             \includegraphics[width=\textwidth]{Figures/Appendix/phewwidth300.png}
%         \end{subfigure}
%           \centering
%         \begin{subfigure}[b]{0.245\textwidth}
%             \centering
%             \includegraphics[width=\textwidth]{Figures/Appendix/phewwidth400.png}
%         \end{subfigure}
%           \centering
%         \begin{subfigure}[b]{0.6\textwidth}
%             \centering
%             \includegraphics[width=\textwidth]{Figures/Appendix/label1.png}
%         \end{subfigure}
%    \caption{\textbf{Effectiveness of bidirectional random walks:} Comparison of bidirectional random walks in PHEW with two variants of unidirectional random walks.}
%    \label{One-DirectionalPHEW}
%\end{figure*}

\subsection{PHEW and path kernel trace}\label{phewpktrace}

Consider a fully-connected MLP with $L$ layers and $N_l$ units per layer.
We consider the Kaiming weight initialization method \cite{he2015delving}, i.e., the initial weight from unit $j$ at layer $l-1$ to unit $i$ at layer $l$ is $\theta^{[l]}(i,j) \thicksim \mathcal{N}(0,\sigma_l^2)$, where $\sigma_l^2 = 2/N_l$.

Consider a path $p$ formed by the edge weights $\{\theta_p^{[l]}\}_{l=1}^L$.
The expected value of the contribution of $p$ to the path kernel trace of the network is:
\begin{equation}
    \mathbb{E}[\bm{\Pi_\theta}(p,p)] = \mathbb{E}\left[\sum_{l=1}^L \left(\dfrac{\pi_p(\theta)}{\theta_p^{[l]}}\right)^2\right] 
\end{equation}
Because the connections that form a path are selected from independent distributions, we can re-write the expectation as,
\begin{equation}
\begin{aligned}
    &\mathbb{E}[\bm{\Pi_\theta}(p,p)] = \sum_{l=1}^L \left[\prod_{i=1,i\neq l}^L \mathbb{E}[\theta_p^{[i]}]^2\right] \\
    & = \sum_{l=1}^L \left[\prod_{i=1,i\neq l}^L \left( \sum_{k=1}^{N_i} \theta^{[i]}(k,j)^2 p^{[i]}(k,j)  \right)\right]
\end{aligned}
\end{equation}
where $\theta^{[i]}(k,j)$ is the edge weight from unit $j$ in layer $i-1$ to unit $k$ in layer $i$ and $p^{[i]}(k,j)$ is the probability of the random walk selecting the edge. 

\textbf{Uniform random walks:} First, suppose that the random walks are not biased. Denote an unbiased path by $p_u$. Then, $p^{[i]}(k,j) = 1/N_i$, and so
\begin{equation}
    \mathbb{E}[\bm{\Pi_\theta}(p_u,p_u)] = \sum_{l=1}^L \left[\prod_{i=1,i\neq l}^L \left( \sum_{k=1}^{N_i} \theta^{[i]}(k,j)^2 \dfrac{1}{N_i}  \right)\right]
\end{equation}
We approximate the values of $\theta^{[i]}(k,j)$ by their expectation based on Kaiming's initialization:
\begin{equation}
    \mathbb{E}[\bm{\Pi_\theta}(p_u,p_u)] \approx \sum_{l=1}^L \left[\prod_{i=1,i\neq l}^L \sigma_i^2\right]
\end{equation}

\textbf{PHEW random walks:} Second, consider a path $p_b$ that is sampled using the PHEW biased random walk process. The previous path kernel trace contribution becomes: $\mathbb{E}[\bm{\Pi_\theta}(p_b,p_b)]=$ 
\begin{equation}
     \sum_{l=1}^L \left[\prod_{i=1,i\neq l}^L \left( \sum_{k=1}^{N_i} \theta^{[i]}(k,j)^2 \dfrac{|\theta^{[i]}(k,j)|}{\sum_{t=1}^{N_i} |\theta^{[i]}(t,j)|}  \right)\right]
\end{equation}
The denominator is the same for all $k=1,...,N_i$. Therefore, 
\begin{equation}
     =\sum_{l=1}^L \left[\prod_{i=1,i\neq l}^L \left( \dfrac{\dfrac{1}{N_i}\sum_{k=1}^{N_i}|\theta^{[i]}(k,j)|^3}{\dfrac{1}{N_i}\sum_{t=1}^{N_i} |\theta^{[i]}(t,j)|}  \right)\right]
\end{equation}
Similarly, approximating the expected value of this ratio by the ratio of the two means: 
\begin{equation}
    \mathbb{E}[\bm{\Pi_\theta}(p_b,p_b)] \approx \sum_{l=1}^L \left[\prod_{i=1,i\neq l}^L \left( \dfrac{2\sqrt{\dfrac{2}{\pi}}\sigma_i^3N_i}{\sqrt{\dfrac{2}{\pi}}\sigma_iN_i}  \right)\right]
\end{equation}
and so,
\begin{equation}
    \mathbb{E}[\bm{\Pi_\theta}(p_b,p_b)] \approx 2^{L-1}\sum_{l=1}^L \left[\prod_{i=1,i\neq l}^L \sigma_i^2\right]
\end{equation}

Therefore, the PHEW biased random walk process creates much larger path kernel trace than unbiased (uniform) random walks, especially in deep networks,
\begin{equation}
    \mathbb{E}[\bm{\Pi_\theta}(p_b,p_b)] = 2^{L-1} \times \mathbb{E}[\bm{\Pi_\theta}(p_u,p_u)]
\end{equation}
