# Supplementary material for: PHEW: Constructing Sparse Networks that Learn Fast and Generalize Well without Training Data
Source: arXiv:2010.11354 source file (2021-06-23)
Supplement: Supplementary file 6 [file Num_Paths2.tex]

\subsection{MLP architecture with maximum number of paths}\label{sec-numpaths}

\textit{Given a target density $\rho$, the maximum number of paths results when each hidden-layer has the same number of units, and the network is fully-connected.}

\textbf{Proof:} We constraint that all  input units must have at least one outgoing connection and all  output units must have at least one incoming connection. 

Let us consider an $L$ layer ReLU network, $f:\R^D\rightarrow \R^K$, with $N_l$ hidden layer units, where $l=1,...,L-1$ .
Let the number of connections in the unpruned network be $M$, 
and the number of  remaining connections after pruning be $m$, according to the target network density $\rho=m/M$.

For simplicity, assume that $m$ is such that we can form a fully-connected network with $n$ hidden units at each layer.
We show next, using induction, that this architecture achieves the maximum number of input-output paths.

\textbf{One hidden layer:} Suppose that the network has one hidden layer with $N$ units.
Let the number of incoming and outgoing connections for hidden unit $i$ be $\{d_i,k_i\}_{i=1}^N$. 
Then the number of paths is given by $P = \sum_{i=1}^N d_i\times k_i$.

Suppose we can identify two hidden units $X$ and $Y$ that are not fully-connected. The number of paths through $X$ is $P(X) = d_x \times k_x$ -- and similarly for $Y$, $P(Y) = d_y \times k_y$. If $P(Y)>P(X)$ we move an edge from $X$ to $Y$ such that the edge is selected from either $d_x$ or $k_x$, choosing the larger among the two. Similarly, the edge is added to either $d_y$ or $k_y$, choosing the smaller among the two. This process causes the number of paths to strictly increase, that is, $\Delta P = max\{d_y,k_y\} - min\{d_x,k_x\} > 0$. In the case of a tie, if $P(X)=P(Y)$, we select the unit with the higher number of incoming/outgoing edges so that $max\{d_y,k_y\} \geq min\{d_x,k_x\}$. If there are still ties, we break them deterministically, moving edges from lower-index units to higher-index units.

We can repeat this process, increasing the number of input-output paths in each iteration, until we cannot find any units that are not fully-connected. Then, the network will consist of $n \leq N$ fully-connected hidden layer units.

\textbf{Two hidden layers:} Let us now consider a network with two hidden layers. We know that the maximum number of paths result when $n_1$ units are active in the first layer and $n_2$ units are active in the second hidden layer such that the network is fully connected. We now show that $n_1=n_2=n$. 

Let us assume that $D=K$. We can make this assumption without the loss of generality because the two sets of input and output units can be partitioned into equal-size subsets with cardinality the highest common factor of the two sets. 
%Intersection of any two subsets is a null set, maximizing the number of paths from all such sets of input units to all sets of output units is equivalent to maximizing the total number of input-output paths.

\begin{equation}
    \argmax_{n_1,n_2} D^2\times n_1 \times n_2, \; s.t \; m = D( n_1 +  n_2 ) + n_1 n_2 
\end{equation}
Substituting for $n_2$ from the constraint, 
\begin{equation}
   \argmax_{n_1} D^2 \times n_1 \times \dfrac{m-Dn_1}{D+n_1}
\end{equation}
Differentiating the equation and equating it to $0$, we obtain $n_1 = -D + \sqrt{D^2+m}$. Similarly, substituting and solving for $n_2$ we obtain $n_2 = -D + \sqrt{D^2+m} = n_1$.Therefore, the number of paths is maximized by having the same number of units $n = n_1 = n_2$ in the two hidden layers.

\textbf{L layers: } The induction hypothesis on a network with $L-1$ layer is: given the target number of connections $m$, the number of paths for a network with $L-1$ layers is maximized by considering a fully-connected network with the same number of units in each of the hidden layer, $n\leq N_i, i=1,...,L-2$, and $m = n(D+K+(L-1)n)$.

Consider now a network with $L$ layers. 
From the induction hypothesis we know that the number of paths $P_{L-2}$ till the last hidden layer  is maximized when each hidden layer contains the same number of units $n$ and is fully-connected. 
All the units in layer $L-2$ have the same number of incoming paths $P_{L-2}/n$.

Suppose that the number of selected units in the last hidden layer is $n_{L-1}\leq N_{L-1}$.
%Now consider the last hidden layer and the output layer, we can equate it to a network with one hidden layer. 
The number of paths $P = \sum_{i=1}^{n} P_{i}\times P_{L-1}/n = P_{L-1}/n\times \sum_{i=1}^{n} P_{i}$, where $P_i$ is the number of paths from $i^{th}$ unit in layer $L-2$ to the output units. 
Using the same proof as the single hidden layer network we can see that $P$ is maximized when $n_{L-1} = n$.

%Therefore, given a target number of connections $m$, the number of input-output paths is maximized by a sub-network such that it has the same number of active units $n$ in all the hidden layers and the sub-network is fully-connected.
